# Supplementary material for: 3D-Printed Sheet Jet for Stable Megahertz Liquid Sample Delivery at X-ray Free Electron Lasers
Source: arXiv:2306.07626 ancillary file (2023-06-13)
Supplement: Supplementary file 1 [file SupplementaryInfo.pdf]

# Supporting Information

## 3D-Printed Sheet Jet for Stable Megahertz Liquid Sample Delivery at X-ray Free Electron Lasers

**Patrick E. Konold *et al.***

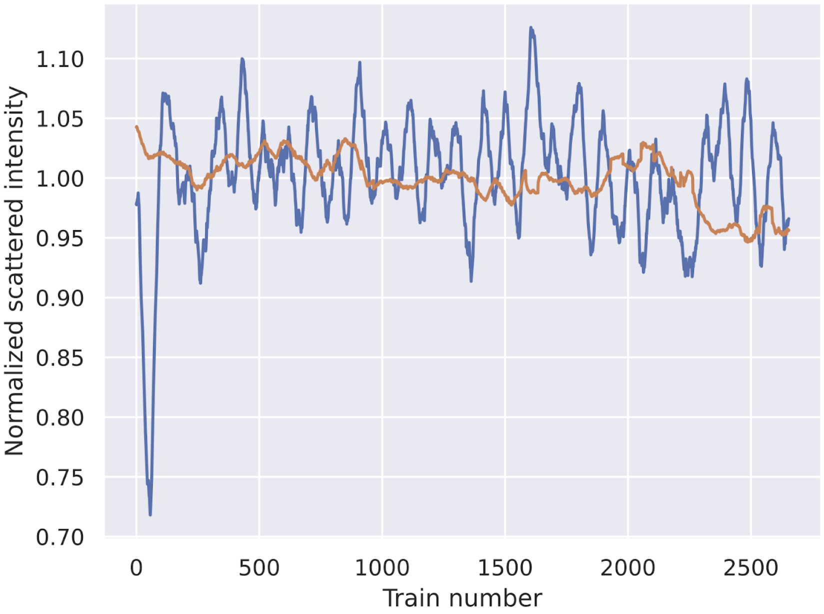


**Figure S1.** The integrated AGIPD detector response normalized by incoming X-ray intensity binned in 50 train intervals over a representative 5 minute measurement window for the liquid sheet jet and GDVN

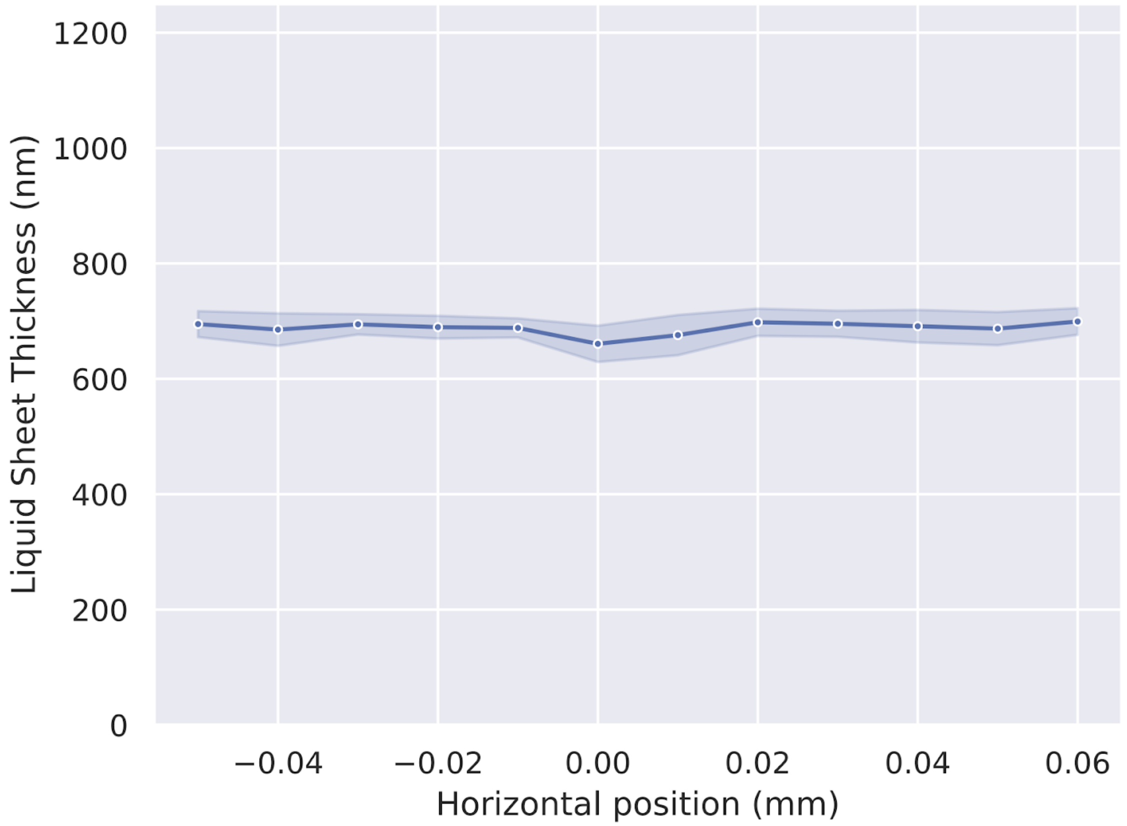


**Figure S2.** Thickness values extracted from scanning horizontally across the primary liquid sheet region at a distance of 185 μm from the nozzle tip.

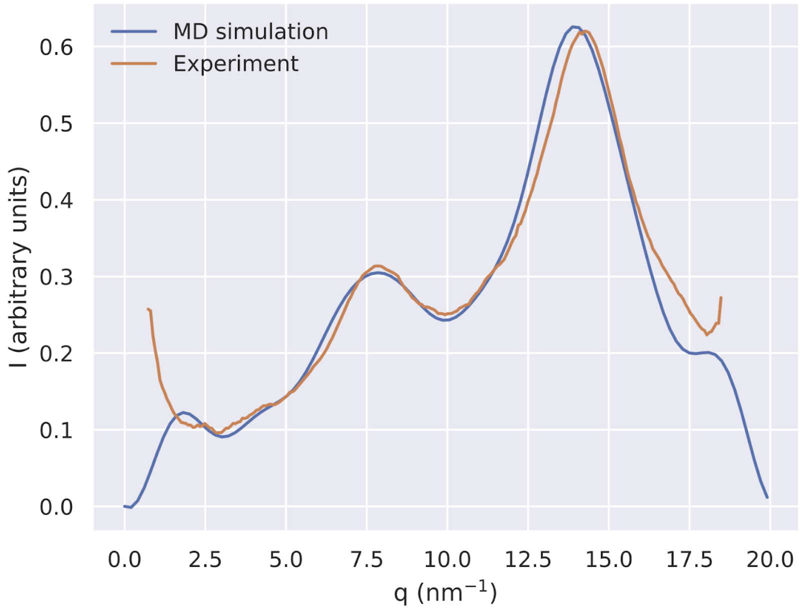


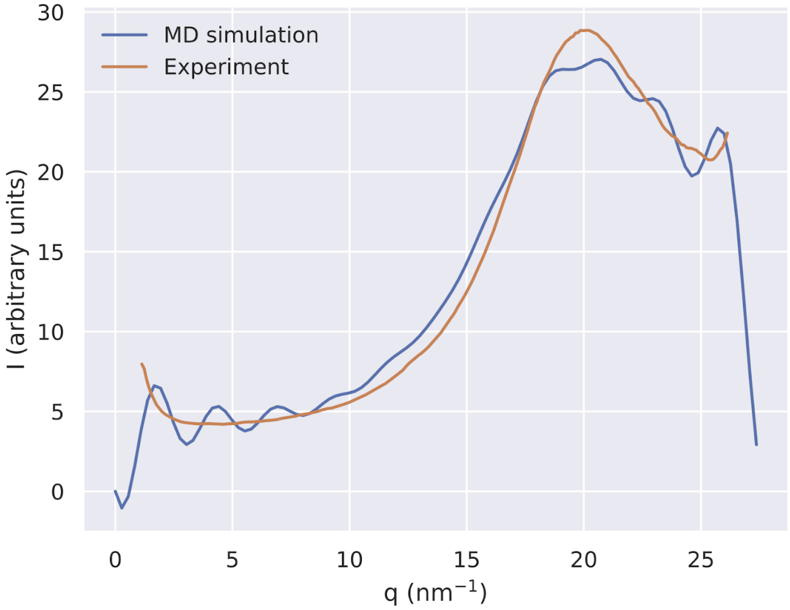


**Figure S3.** Scattering curves derived from molecular dynamics simulations. Above for isopropanol delivered by the liquid sheet and below for water delivered by a GDVN.

**Movie S1.** run 194

**Movie S2.** run 186
